# Supplementary material for: Magnetic phase diagram of La$_{2-x}$Sr$_{x}$CoO$_{4}$ revised using muon-spin relaxation
Source: arXiv:1510.06244 source file (2015-10-21)
Supplement: Supplementary file 1 [file supplemental.pdf]

# Supplemental Material: Magnetic phase diagram of $La_{2-x}Sr_xCoO_4$ revised using muon-spin relaxation


R. C. Williams,[1] F. Xiao,[1] T. Lancaster,[1] R. De Renzi,[2] G. Allodi,[2] S. Bordignon,[2] P. G. Freeman,[3,4,*] F. L. Pratt,[5] S. R. Giblin,[6] J. S. Möller,[7,†] S. J. Blundell,[7] A. T. Boothroyd,[7] and D. Prabhakaran[7]

[1] *Centre for Materials Physics, Durham University, Durham, DH1 3LE, United Kingdom*

[2] *Dipartimento di Fisica e Scienze della Terra, Università degli Studi di Parma, Viale delle Scienze 7A, I-43124 Parma, Italy*

[3] *École Polytechnique Fédérale de Lausanne, ICMP, Lab Quantum Magnetism, CH-1015 Lausanne, Switzerland*

[4] *Institut Laue-Langevin, 71 avenue des Martyrs 38000 Grenoble, France*

[5] *ISIS Facility, STFC Rutherford Appleton Laboratory, Chilton, Didcot, Oxfordshire, OX11 0QX, United Kingdom*

[6] *School of Physics and Astronomy, Cardiff University, Queen's Buildings, The Parade, Cardiff, CF24 3AA, United Kingdom*

[7] *Oxford University Department of Physics, Clarendon Laboratory, Parks Road, Oxford, OX1 3PU, United Kingdom*



(Dated: October 21, 2015)


## SAMPLE SYNTHESIS

Polycrystalline $La_{2-x}Sr_xCoO_4$ (LSCO), $x = 0$ to 0.9, powder samples were prepared from the stoichiometric amount of high purity ($> 99.99\%$) $La_2O_3$, $SrCO_3$ and $Co_3O_4$. Lower doped ($x < 0.1$) samples were sintered at 1100°C and 1150°C for 48 h with intermediate grinding under a flowing atmosphere of high purity argon. For higher doped samples ($x > 0.1$), powders were sintered at 1200°C with intermediate grinding under flowing atmospheres of high purity argon ($0.15 < x < 0.2$), argon plus oxygen ($0.25 < x < 0.5$) or oxygen ($0.67 < x < 0.9$) for 72 h. All the powder samples were checked for impurity phases using x-ray powder diffraction. Single phase powders were isostatically pressed into cylindrical rods of diameter 10 mm and length 10 cm. The rods were sintered at 1250°C for 24 h under flowing atmospheres of $CO/CO_2$ mixed in the ratio $2 : 10$ for $x < 0.1$, and similar atmospheres as before for $x > 0.15$. Single crystals were grown using a four mirror optical floating-zone furnace at a growth speed of 1–2 mm/h with counter-rotation of the feed and seed rods at 25 rpm under a similar atmosphere as that of final sintering.

## EXPERIMENTAL PROCEDURE

In a $\mu^+$SR experiment [1] spin-polarized positive muons are implanted into the sample and subsequently decay into a positron with average lifetime $\tau = 2.2$ μs. The decay positron is emitted preferentially in the direction of the muon's instantaneous spin vector. Detectors grouped Forward (F) and Backward (B) with respect to the muon beam's initial spin polarization direction allow one to measure the positron asymmetry

$$A(t) = \frac{N_{\mathrm{F}}(t) - \alpha N_{\mathrm{B}}(t)}{N_{\mathrm{F}}(t) + \alpha N_{\mathrm{B}}(t)}, \tag{1}$$

where $N_{\mathrm{F,B}}(t)$ are the event histograms at a time $t$ after the muon implantation, and $\alpha$ is an experimental calibration constant. The asymmetry $A(t)$ is proportional to the muon ensemble's spin polarization, the time-dependence of which is sensitive to the local magnetic field experienced at the muons' stopping sites.

A range of investigations have been conducted regarding the location of the muon stopping site in the cuprate system $La_{2-x}Sr_xCuO_4$, by considering magnetic dipole field arising from magnetic and nuclear moments, electrostatic potential landscapes and and *ab initio* calculations. The broad consensus is that the muon is believed to come to rest near the apical oxygen of the $CuO_6$ octahedra [2–6]. It may be expected that the muon behaves similarly in the LSCO series. It is possible to show [7] that the depolarization of an implanted muon is sensitive to field correlations $\Phi_{ii}$ where $i$ are directions in the plane perpendicular to the initial direction of the muon polarization $\boldsymbol{P}(t = 0)$. In our experiments $\boldsymbol{P}(t = 0)$ is parallel to the crystallographic $c$-axis of the tetragonal unit cell, and therefore $i$ are directions in the $ab$-plane. Magnetic moments in ordered state are also confined within the $ab$-plane, however, since muons couple to dipole fields, the field and spin directions do not generally coincide.

## FURTHER DETAILS OF DATA ANALYSIS

In order to probe the dynamics of the system LSCO across the phase diagram all datasets were fitted to the stretched exponential relaxation function

$$A(t) = A_{\mathrm{rel}} e^{-(\lambda t)^{\beta}} + A_{\mathrm{b}}, \tag{2}$$

where $A_{\mathrm{rel}}$ and $A_{\mathrm{b}}$ are the relaxing and non-relaxing baseline amplitudes, respectively and $\beta$ was constrained to be greater than 0.5. This phenomenological expression is a versatile relaxation function, able to characterize a broad

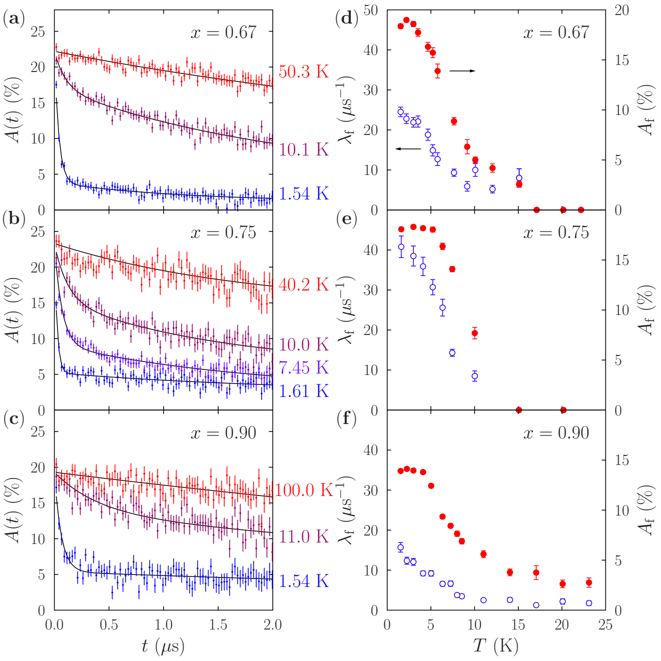


FIG. S1: (a)–(c) Example asymmetry spectra from compounds in Region III ($x$ = 0.67, 0.75 and 0.9), measured at S$\mu$S. Solid lines are fits (see main text) (d)–(f) Amplitude and relaxation rates of the fast relaxing components.

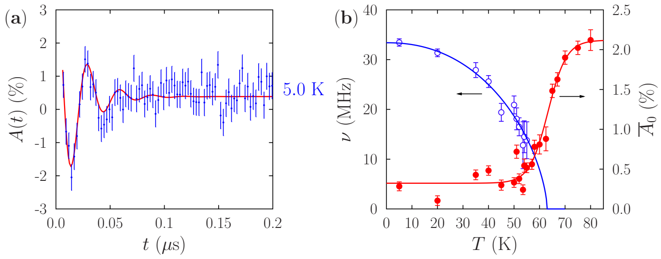


FIG. S2: (a) Example asymmetry data for $La_{2-x}Sr_xNiO_4$ measured at 5 K on the DOLLY instrument at S$\mu$S. Solid line is a fit (see text) (b) Fitted precession frequency, and early-time average asymmetry. Red line is a fit (see text), and blue line is a guide to the eye.

range of decaying curve shapes and extract a representative relaxation rate $\lambda$. This fitting routine was found to capture the same qualitative features at the same temperatures as more complex fitting routines involving sums of exponential and Gaussian terms, which have a more physical basis. The versatility of the stretched exponential term allows direct comparisons to be made for the data measured across the entire $x$-$T$ plane of the phase diagram.

The data were binned into time intervals of $\Delta t$ = 16.0 ns for ISIS data (the highest resolution available) and 3.91 ns for S$\mu$S data, for which the greatest available resolution is $\Delta t = 0.977$ ns ($\Delta t = 9.77$ ns was used for the S$\mu$S data for $x = 0.9$ to account for the lower statistic datasets). This serves to average out the oscillations visible in $A(t)$ for low times in S$\mu$S data for samples below $T_N$, and hence reduce their impact on the coarser fit.

## Region III

Asymmetry data for compounds within region III [$x$ = 0.67, 0.75 and 0.9, example spectra shown in Fig. S1(a)–(c)] were found to be best fitted to a purely relaxing asymmetry function comprising two exponentially decaying components plus a non-relaxing background contribution: $A(t) = A_f e^{-\lambda_f t} + A_s e^{-\lambda_s t} + A_b$, where the initial asymmetry $A_0 = A_f + A_s + A_b$ was fixed to the high-$T$ value of $\overline{A}_0$ for each compound ($\lambda_s$ was fixed to its average value of 0.13 MHz for $x = 0.90$). Plotted parameters for the amplitude and relaxation rate of the fast decaying term are shown in Fig. S1(d)–(f).

## $La_{2-x}Sr_xNiO_4$

$La_{2-x}Sr_xNiO_4$ (LSNO) is another non-superconducting cousin of the cuprates, where the appearance of stripe CO is well established [8, 9], although the hole-carrying $Ni^{3+}$ ions still possess a magnetic spin, and therefore interact with one another and the $Ni^{2+}$ ions. Muon data measured on $x = 0.5$ LSNO, using the DOLLY instrument at S$\mu$S, are qualitatively similar to that of the equivalent LSCO compound; Heavily damped oscillations, indicating quasistatic SO, are visible in asymmetry data below around 60 K, shown in Fig. S2(a).

Early-time average asymmetry $\overline{A}_0$ is shown in Fig. S2(b), and a fit to the broadened step function (see main text) yields a transition temperature $T_N$ = 63(4) K, similar to that obtained in previous studies [10, 11]. Asymmetry datasets showing spontaneous precesssion frequencies were fitted for $t \leq 1$ $\mu$s to $A(t) = A_{osc}\cos(2\pi\nu t)e^{-\lambda_{osc}t} + A_{rel}e^{-\lambda_{rel}t}$, where the amplitude of the oscillatory term was fitted to its average value of $A_{osc}$ = 4.5%. The single frequency oscillatory component comprises nearly all of the asymmetry amplitude in the ordered phase, which suggests there is no phase separation within the sample. However, large values of the transverse relaxation rate $\lambda_{osc}$ suggest a broad field distribution is experienced by the muon ensemble.

The fitted precession frequencies are shown in Fig. S2(b), however the transverse relaxation rate $\lambda_{osc}$ increases as temperatures approach $T_N$ from below, and oscillations cease to be resolvable for $T \gtrsim 55$ K. It is interesting to note that magnetic order on the muon time scale appears around the same temperature as a spin reorientation is observed by neutron diffraction measurements [12].

---

* Present address: Jeremiah Horrocks Institute, University of Central Lancashire, Preston PR1 2HE, United Kingdom

† Present address: Neutron Scattering and Magnetism, Laboratory for Solid State Physics, ETH Zürich, CH-8093 Zürich, Switzerland

[1] S. J. Blundell, Contemp. Phys. **40**, 175 (1999).
[2] B. Hitti, P. Birrer, K. Fischer, F. N. Gygax, E. Lippelt, H. Maletta, A. Schenck, and M. Weber, Hyperfine Interact. **63**, 287 (1990).
[3] E. Torikai, K. Nagamine, H. Kitazawa, I. Tanaka, H. Kojima, S. B. Sulaiman, S. Srinivas, and T. P. Das, Hyperfine Interact. **79**, 921 (1993).
[4] S. B. Sulaiman, S. Srinivas, N. Sahoo, F. Hagelberg, T. P. Das, E. Torikai, and K. Nagamine, Phys. Rev. B **49**, 9879 (1994).
[5] B. Nachumi, Y. Fudamoto, A. Keren, K. Kojima, M. Larkin, G. M. Luke, J. Merrin, O. Tchernyshyov, Y. J. Uemura, N. Ichikawa, M. Goto, H. Takagi, S. Uchida, M. K. Crawford, E. M. McCarron, D. E. MacLaughlin, and R. H. Heffner, Phys. Rev. B **58**, 8760 (1998).
[6] W. Huang, V. Pacradouni, M. P. Kennett, S. Komiya, and J. E. Sonier, Phys. Rev. B **85**, 104527 (2012).
[7] T. McMullen and E. Zaremba, Phys. Rev. B **18**, 3026 (1978).
[8] C. H. Chen, S.-W. Cheong, and A. S. Cooper, Phys. Rev. Lett. **71**, 2461 (1993).
[9] V. Sachan, D. J. Buttrey, J. M. Tranquada, J. E. Lorenzo, and G. Shirane, Phys. Rev. B **51**, 12742 (1995).
[10] Th. Jestädt, K. H. Chow, S. J. Blundell, W. Hayes, F. L. Pratt, B. W. Lovett, M. A. Green, J. E. Millburn, and M. J. Rosseinsky, Phys. Rev. B **59**, 3775 (1999).
[11] K. H. Chow, P. A. Pattenden, S. J. Blundell, W. Hayes, F. L. Pratt, Th. Jestädt, M. A. Green, J. E. Millburn, M. J. Rosseinsky, B. Hitti, S. R. Dunsiger, R. F. Kiefl, C. Chen, and A. J. S. Chowdhury, Phys. Rev. B **53**, R14725 (1996).
[12] P. G. Freeman, A. T. Boothroyd, D. Prabhakaran, D. González, and M. Enderle, Phys. Rev. B 66, 212405 (2002).
